# Supplementary material for: Converging Divergent Paths: Constant Charge vs. Constant Potential Energetics in Computational Electrochemistry
Source: arXiv:2312.00911 ancillary file (2023-12-01)
Supplement: Supplementary file 1 [file si.pdf]

# Supporting Information

## Converging Divergent Paths: Constant Charge vs. Constant Potential Energetics in Computational Electrochemistry

Nicolas G. Hörmann,[*,†] Simeon D. Beinlich,[†,‡] and Karsten Reuter[†]

†*Fritz-Haber-Institut der Max-Planck-Gesellschaft, Faradayweg 4-6, 14195 Berlin, Germany.*

‡*Technical University of Munich, Lichtenbergstr. 4, 85747 Garching, Germany*

E-mail: hoermann@fhi.mpg.de

# S1 Equivalence of Canonical Energy Differences at Constant Field and Constant surface Excess Charge

Originally, the canonical, constant charge (CC) CHE approach models the applied potential by simulating the interfacial system at a fixed interfacial electrostatic field **E** which can be simulated in density functional theory calculations by introducing an external saw-tooth potential.[1,2] Similarly, an interfacial field **E** can be created by adding appropriate excess atoms into the interfacial region which donate or remove electrons to/from the surface. As an example, H atoms placed into interfacial water will donate a (partial) electron to the metallic surface and transform into a (partially charged) excess proton in interfacial water – a charge configuration which naturally sets up an interfacial field.[3,4] In more recent simulations in implicit solvent environments, it is as well possible to setup an interfacial field by simply varying the number of (excess) electrons $N_{e^-}^{\mathrm{net}}$[5–7] which naturally induces charge-compensating electrolyte counter charges within the implicit solvent model and thereby allows to create an interfacial field **E**.

Let us consider the latter type of methods and the case that only Hydrogen adsorbates exist. In this case one can write a straight forward Taylor expansion of the canonical CC Gibbs energy of the surface $G^{\mathrm{s}}$ around the charge neutral point (potential of zero charge, PZC) where $N_{e^-}^{\mathrm{net}} = 0$.[8,9] In particular, the linear order change of $G^{\mathrm{s}}$ with $N_{e^-}^{\mathrm{net}}$ simply reads

$$G^{\mathrm{s}}(N_{\mathrm{H}}, N_{e^-}^{\mathrm{net}}) \approx G^{\mathrm{s,PZC}}(N_{\mathrm{H}}) + N_{e^-}^{\mathrm{net}} \tilde{\mu}_{e^-}^{\mathrm{PZC}}(N_{\mathrm{H}}) \ , \tag{S1}$$

from the basic thermodynamic definition of the electron electrochemical potential at the PZC $\tilde{\mu}_{e^-}^{\mathrm{PZC}} = \frac{\partial G^{\mathrm{s}}}{\partial N_{e^-}^{\mathrm{net}}}\Big|_{\mathrm{PZC}}$. As a result one obtains for the energy change with respect to the number of hydrogen adsorbates $N_{\mathrm{H}}$ at given $N_{e^-}^{\mathrm{net}}$

$$\frac{\mathrm{d}G^{\mathrm{s}}}{\mathrm{d}N_{\mathrm{H}}}\bigg|_{N_{e^-}^{\mathrm{net}}} \approx \frac{\mathrm{d}G^{\mathrm{s}}}{\mathrm{d}N_{\mathrm{H}}}\bigg|_{\mathrm{PZC}} + N_{e^-}^{\mathrm{net}} \frac{\mathrm{d}\tilde{\mu}_{e^-}^{\mathrm{PZC}}}{\mathrm{d}N_{\mathrm{H}}} \ . \tag{S2}$$

Evidently the last term in eq. S2 has the identical structure as a dipole-field interaction[10] $-\mathbf{ED}$ with $\mathbf{E} = -\frac{eN_{e^-}^{\mathrm{net}}}{\epsilon_0 A}$ the average interfacial field and $\mathbf{D} = \frac{\epsilon_0 A}{e}\frac{\mathrm{d}\tilde{\mu}_{e^-}^{\mathrm{PZC}}}{\mathrm{d}N_{\mathrm{H}}}$ the adsorbate dipole as deduced from the adsorbate-induced work function change $\frac{\mathrm{d}\Phi_0}{\mathrm{d}N_{\mathrm{H}}} = -\frac{\mathrm{d}\tilde{\mu}_{e^-}^{\mathrm{PZC}}}{\mathrm{d}N_{\mathrm{H}}}$ which relates to a change in the potential drop across the inner double layer of $\frac{\mathrm{d}\phi_0}{\mathrm{d}N_{\mathrm{H}}} = \frac{1}{e}\frac{\mathrm{d}\Phi_0}{\mathrm{d}N_{\mathrm{H}}}$.[1] Hence CC calculations at finite net charge $N_{e^-}^{\mathrm{net}} \neq 0$ show a behavior consistent with a dipole-field interaction, which could be equally probed by DFT calculations in a field $\mathbf{E}$. Thus, at an appropriately chosen field strength $\mathbf{E}$, constant field calculations are expected to yield identical results to constant charge calculations as e.g. demonstrated in Ref. 11.

# S2 Relation between Constant Charge and Constant Potential Descriptions

In perfect analogy to the procedures described in Ref. 12 the application of the chain rule to a total differential yields

$$\left.\frac{\mathrm{d}G^{\mathrm{s}}}{\mathrm{d}N_{\mathrm{H}^+}}\right|_{\tilde{\mu}_{e^-}} = \left.\frac{\partial G^{\mathrm{s}}}{\partial N_{\mathrm{H}^+}}\right|_{N_{e^-}(\tilde{\mu}_{e^-})} + \left.\frac{\partial G^{\mathrm{s}}}{\partial N_{e^-}}\right|_{N_{\mathrm{H}^+}} \left.\frac{\partial N_{e^-}}{\partial N_{\mathrm{H}^+}}\right|_{\tilde{\mu}_{e^-}} \tag{S3}$$

$$\overset{\text{eq. 8}}{=} \left.\frac{\partial G^{\mathrm{s}}}{\partial N_{\mathrm{H}^+}}\right|_{N_{e^-}(\tilde{\mu}_{e^-})} + \left.\frac{\partial G^{\mathrm{s}}}{\partial N_{e^-}}\right|_{N_{\mathrm{H}^+}} + \left.\frac{\partial G^{\mathrm{s}}}{\partial N_{e^-}}\right|_{N_{\mathrm{H}^+}} \left.\frac{\partial N_{e^-}^{\mathrm{net}}}{\partial N_{\mathrm{H}^+}}\right|_{\tilde{\mu}_{e^-}} \tag{S4}$$

$$= \left.\frac{\mathrm{d}G^{\mathrm{s}}}{\mathrm{d}N_{\mathrm{H}}}\right|_{N_{e^-}^{\mathrm{net}}(\tilde{\mu}_{e^-})} + \left.\frac{\partial G^{\mathrm{s}}}{\partial N_{e^-}}\right|_{N_{\mathrm{H}^+}} \left.\frac{\partial N_{e^-}^{\mathrm{net}}}{\partial N_{\mathrm{H}^+}}\right|_{\tilde{\mu}_{e^-}} \tag{S5}$$

$$= \left.\frac{\mathrm{d}G^{\mathrm{s}}}{\mathrm{d}N_{\mathrm{H}}}\right|_{N_{e^-}^{\mathrm{net}}(\tilde{\mu}_{e^-})} + \tilde{\mu}_{e^-} \left.\frac{\partial N_{e^-}^{\mathrm{net}}}{\partial N_{\mathrm{H}^+}}\right|_{\tilde{\mu}_{e^-}} \tag{S6}$$

from the identity $\frac{\partial G^{\mathrm{s}}}{\partial N_{e^-}} = \tilde{\mu}_{e^-}$ at equilibrium. Eq. S6 is eq. 9 of the main text.

[1]Note that we use the standard conventions for measuring energies and potentials: $\tilde{\mu}_{e^-}$ is thereby on a normal energy scale (more negative values for electrons that are stronger bound to the electrode) while work function and electrode potentials are measured on an inverse scale (more positive values for electrons that are stronger bound to the electrode). Furthermore, for the definition of the dipole $\mathbf{D}$ we use the physics sign convention, in contrast to previous works.[10]

# S3 Size Dependence of CC Energy Differences: Details on Fig. 1 of the Manuscript

Fig. 1 of the main text reports on the size dependence for the energy difference $\Delta_A E^{\mathrm{DFT}}$ between a desorbed and an adsorbed proton. The upper panel reports in particular the value $\Delta_A E^{\mathrm{DFT}} - \Delta_\infty E^{\mathrm{DFT}}$ in order to concentrate only on the size-dependent part of $\Delta_A E^{\mathrm{DFT}}$.

The literature datapoints (dots, Chan2015) were obtained from Table 1 in Ref. 13, which reports the work function ($\Phi_{\mathrm{FS}}$- $\Phi_{\mathrm{IS}}$) as well as the energy difference ($E_{\mathrm{FS}}$- $E_{\mathrm{IS}}$) between final state (FS) and initial (IS) for a proton adsorption reaction (Volmer step) for different cell sizes on Pt(111). In order to obtain the here reported differences between desorbed and adsorbed proton ('IS-FS') the work function and energy data of Chan was multiplied by a factor of $-1$ to obtain values in our nomenclature ($\Delta_A \phi_0 = -\frac{1}{e}(\Phi_{\mathrm{FS}} - \Phi_{\mathrm{IS}})$, $\Delta_A E^{\mathrm{DFT}} = -(E_{\mathrm{FS}} - E_{\mathrm{IS}})$).

Note, furthermore, that the (signs in the) plate capacitor energetics as described here only applies for extrapolation to the FS which is why we only concentrate on the data 'Volmer, to FS' and 'Volmer, 1ML *H'. However, if signs are ignored, magnitude and scaling laws of the CC size dependence are very similar also for other considered reaction steps and extrapolation endpoints (Fig. 3 in Ref. 13), due to the generic electrostatics they derive from.

Our own data is obtained by explicit, standard DFT calculations of a desorbed and and adsorbed proton in charge neutral DFT cells on top of a Au(111) surface in implicit solvent environment. In the desorbed state ($* + e^- + H^+ + nH_2O$; for convenience ($* + e^-$) is not mentioned explicitly in the following), the proton is solvated explicitly by a single explicit $H_2O$ molecule in the interfacial region, or by a water cluster of three $H_2O$ molecules connected by hydrogen bonds. The adsorbed state is treated with an according explicit solvation environment. DFT energies were evaluated for the desorbed state ($H^+$ & $H_2O$, $H^+$ & $H_2O$ cluster) and the adsorbed state (*H & $H_2O$, *H & $H_2O$ cluster) at various sizes of the hexagonal supercell ($3 \times 3$, $6 \times 3$, and $6 \times 6$). More computational details are provided

below in section S4.

The supercells are extrapolated to three different states by adding cells with different surface configurations (labelling as in Fig. 1 of the main text):

- $H^+$ & $H_2O \overset{\infty}{\rightarrow}$ 0.11 ML (*H & $H_2O$):

  *Extrapolation to the covered surface (H coverage of 1/9), with adjacent $H_2O$.*

  Consistent with the established size-extrapolation schemes,[13] the desorbed state in the bigger cells is modelled with one desorbed proton (and solvating $H_2O$), while keeping the surrounding in an adsorbed proton state configuration (and solvating $H_2O$). This keeps thus the coverage of solvating $H_2O$ always constant at 0.11 ML and extrapolates to the 0.11 ML (*H & $H_2O$) configuration. The same scheme was applied in the calculations with a solvating water cluster.

- $H^+$ & $H_2O \overset{\infty}{\rightarrow}$ 0.11 ML *H:

  *Extrapolation to the covered surface (H coverage of 1/9), no adjacent $H_2O$.*

  The desorbed state in the bigger cells is modelled with one desorbed proton (and solvating $H_2O$), while keeping the surrounding in an adsorbed proton state configuration but removing the solvating $H_2O$ for these adsorbed protons. Here the coverage of solvating $H_2O$ is kept at the coverage of the desorbed proton. This approach extrapolates to the 0.11 ML *H configuration without solvating, explicit waters.

- $H^+$ & $H_2O \overset{\infty}{\rightarrow}$ 0.0 ML *H:

  *Extrapolation to the clean surface (H coverage of 0.0), no adjacent $H_2O$*

  The desorbed state in the bigger cells is modelled with one desorbed proton (and solvating $H_2O$), while removing all atoms in the surrounding. This is the most straight forward extrapolation scheme when it comes to rationalizing the cell size dependence of the desorbed proton energy in CC calculations. Here the coverage of $H_2O$ is always the desorbed proton coverage. This approach extrapolates to the 0.0 ML *H configuration, and thus to the limit of the clean surface without solvating, explicit waters.

In order to obtain the pure finite size effects $\Delta_A E^{\mathrm{DFT}} - \Delta_\infty E^{\mathrm{DFT}}$ reported in Fig. 1. of the main text, we fitted in all cases (literature and own data) a linear function $M \cdot \Delta_A \phi_0 + \Delta_\infty E^{\mathrm{DFT}}$ through the datapoints $\Delta_A E^{\mathrm{DFT}}(\Delta_A \phi_0)$ which yields $\Delta_\infty E^{\mathrm{DFT}}$ and $M = \frac{\partial \Delta_A E^{\mathrm{DFT}}}{\partial \Delta_A \phi_0}$ and leads to Fig. 1 in the main text.

All data and a jupyter notebook including all scripts as described for recreating Fig. 1 of the main text are available at https://doi.org/10.17617/3.6W6BGK.

# S4 Computational Details

We performed Density Functional Theory (DFT) calculations using the Atomic Simulation Environment (ASE)[14] in combination with the GPAW[15,16] DFT code and the Solvated Jellium Model (SJM)[5] as a continuum representation of the electrolyte. The Au(111) electrode was modelled using slabs of four atomic layers thickness (the bottom two layers are frozen in the bulk geometry) and a vacuum region of at least 20 Å thickness.

We employed the Beef-vdW exchange-correlation functional[17] and a spacing of the real space grid of below 0.17 Å, which results in a $48 \times 48 \times 192$ grid for the Au(111) $3 \times 3$ supercell, a $96 \times 48 \times 192$ grid for the $6 \times 3$ supercell, and a $96 \times 96 \times 192$ grid for the $6 \times 6$ supercell. We use Γ-centered Monkhorst-Pack grids in lateral directions (K-points distance of below 0.15 $\text{Å}^{-1}$) and a single K-point in vertical direction yielding a $6 \times 6 \times 1$ K-point grid for the $3 \times 3$ supercell, a $3 \times 6 \times 1$ K-point grid for the $6 \times 3$ supercell, and $3 \times 3 \times 1$ K-point grid for $6 \times 6$ supercell. Fermi-Dirac smearing (width of 0.1eV) and Pulay mixing (linear mixing of 3 previous densities, strength $\beta = 0.05$, and metric weight of 50.0) is applied to improve convergence of the electronic self-consistent-field cycles.

Using these parameters yields a Au lattice constant of 4.275 Å which was determined from a common bulk optimization ($18 \times 18 \times 18$ K-point grid and $16 \times 16 \times 16$ real space grid). All atomic structures are relaxed until the atomic forces are below 0.03 eV/Å using the BFGS algorithm as implemented in ASE.[14]

The surrounding electrolyte is modelled using an implicit solvent setup as implemented in the SJM[5] extension of GPAW[15,16] (linear dielectric constant of 78.36 and surface tension of $1.1484 \cdot 10^{-3}\,\mathrm{eV/\AA^2}$), The implicit-explicit boundary is defined using a *power12potential* (strength 0.18 eV, temperature 298.15 K, Van-der-Waals radii of the Au atoms scaled by a factor of 1.08). The factor for the radius scaling was adjusted such, that when performing calculations at finite excess charge (jellium counter charge at a distance of 3 Å to the highest atom and 1 Å below the dipole-correction layer) the electronic capacitance $19\,\mu\mathrm{F/cm^2}$ and and the PZC of 4.7 V of the clean Au(111) slab match the experimental values of $\approx 15 - 30\,\mu\mathrm{F/cm^2}$ [18] and $\approx 4.9$ V[19,20] on an absolute electrode potential scale. All calculations in this work are performed at zero excess charge q=0, i.e., at the PZC.

# References


(1) Nørskov, J. K.; Rossmeisl, J.; Logadottir, A.; Lindqvist, L.; Kitchin, J. R.; Bligaard, T.; Jónsson, H. Origin of the Overpotential for Oxygen Reduction at a Fuel-cell Cathode. *J. Phys. Chem. B* **2004**, *108*, 17886–17892, DOI: 10.1021/jp047349j.

(2) Kelly, S. R.; Kirk, C.; Chan, K.; Nørskov, J. K. Electric Field Effects in Oxygen Reduction Kinetics: Rationalizing pH Dependence at the Pt(111), Au(111), and Au(100) Electrodes. *J. Phys. Chem. C* **2020**, *124*, 14581–14591, DOI: 10.1021/acs.jpcc.0c02127.

(3) Skúlason, E.; Karlberg, G. S.; Rossmeisl, J.; Bligaard, T.; Greeley, J.; Jónsson, H.; Nørskov, J. K. Density Functional Theory Calculations for the Hydrogen Evolution Reaction in an Electrochemical Double Layer on the Pt(111) Electrode. *Phys. Chem. Chem. Phys.* **2007**, *9*, 3241–3250, DOI: 10.1039/B700099E.

(4) Rossmeisl, J.; Skúlason, E.; Björketun, M. E.; Tripkovic, V.; Nørskov, J. K. Modeling the Electrified Solid–liquid Interface. *Chem. Phys. Lett.* **2008**, *466*, 68–71, DOI: 10.1016/j.cplett.2008.10.024.

(5) Kastlunger, G.; Lindgren, P.; Peterson, A. A. Controlled-potential Simulation of Elementary Electrochemical Reactions: Proton Discharge on Metal Surfaces. *J. Phys. Chem. C* **2018**, *122*, 12771–12781, DOI: 10.1021/acs.jpcc.8b02465.

(6) Gauthier, J. A.; Ringe, S.; Dickens, C. F.; Garza, A. J.; Bell, A. T.; Head-Gordon, M.; Nørskov, J. K.; Chan, K. Challenges in Modeling Electrochemical Reaction Energetics with Polarizable Continuum Models. *ACS Catal.* **2019**, *9*, 920–931, DOI: 10.1021/acscatal.8b02793.

(7) Hörmann, N. G.; Marzari, N.; Reuter, K. Electrosorption at Metal Surfaces from First Principles. *npj Comput. Mater* **2020**, *6*, 1–10, DOI: 10.1038/s41524-020-00394-4.

(8) Hörmann, N. G.; Andreussi, O.; Marzari, N. Grand Canonical Simulations of Electrochemical Interfaces in Implicit Solvation Models. *J. Chem. Phys.* **2019**, *150*, 041730, DOI: 10.1063/1.5054580.

(9) Domínguez-Flores, F.; Melander, M. M. Approximating Constant Potential DFT with Canonical DFT and Electrostatic Corrections. *J. Chem. Phys.* **2023**, *158*, 144701, DOI: 10.1063/5.0138197.

(10) Beinlich, S. D.; Hörmann, N. G.; Reuter, K. Field Effects at Protruding Defect Sites in Electrocatalysis at Metal Electrodes? *ACS Catal.* **2022**, *12*, 6143–6148, DOI: 10.1021/acscatal.2c00997.

(11) Dudzinski, A. M.; Diesen, E.; Heenen, H. H.; Bukas, V. J.; Reuter, K. First Step of the Oxygen Reduction Reaction On Au(111): A Computational Study of O2 Adsorption at the Electrified Metal/water Interface. *ACS Catal.* **2023**, *13*, 12074–12081, DOI: 10.1021/acscatal.3c02129.

(12) Beinlich, S. D.; Kastlunger, G.; Reuter, K.; Hörmann, N. G. A Theoretical Investigation of the Grand- and the Canonical Potential Energy Surface: The Interplay

between Electronic and Geometric Response at Electrified Interfaces. *arXiv* **2023**, arXiv:2307.09817v1 [physics.chem–ph], DOI: 10.48550/ARXIV.2307.09817.

(13) Chan, K.; Nørskov, J. K. Electrochemical Barriers Made Simple. *J. Phys. Chem. Lett.* **2015**, *6*, 2663–2668, DOI: 10.1021/acs.jpclett.5b01043.

(14) Larsen, A. H.; Mortensen, J. J.; Blomqvist, J.; Castelli, I. E.; Christensen, R.; Dułak, M.; Friis, J.; Groves, M. N.; Hammer, B.; Hargus, C.; Hermes, E. D.; Jennings, P. C.; Jensen, P. B.; Kermode, J.; Kitchin, J. R.; Kolsbjerg, E. L.; Kubal, J.; Kaasbjerg, K.; Lysgaard, S.; Maronsson, J. B.; Maxson, T.; Olsen, T.; Pastewka, L.; Peterson, A.; Rostgaard, C.; Schiøtz, J.; Schütt, O.; Strange, M.; Thygesen, K. S.; Vegge, T.; Vilhelmsen, L.; Walter, M.; Zeng, Z.; Jacobsen, K. W. The Atomic Simulation Environment—a Python Library for Working with Atoms. *J. Phys.: Condens. Matter* **2017**, *29*, 273002, DOI: 10.1088/1361-648X/aa680e.

(15) Mortensen, J. J.; Hansen, L. B.; Jacobsen, K. W. Real-space Grid Implementation of the Projector Augmented Wave Method. *Phys. Rev. B* **2005**, *71*, 035109, DOI: 10.1103/PhysRevB.71.035109.

(16) Enkovaara, J.; Rostgaard, C.; Mortensen, J. J.; Chen, J.; Dułak, M.; Ferrighi, L.; Gavnholt, J.; Glinsvad, C.; Haikola, V.; Hansen, H. A.; Kristoffersen, H. H.; Kuisma, M.; Larsen, A. H.; Lehtovaara, L.; Ljungberg, M.; Lopez-Acevedo, O.; Moses, P. G.; Ojanen, J.; Olsen, T.; Petzold, V.; Romero, N. A.; Stausholm-Møller, J.; Strange, M.; Tritsaris, G. A.; Vanin, M.; Walter, M.; Hammer, B.; Häkkinen, H.; Madsen, G. K. H.; Nieminen, R. M.; Nørskov, J. K.; Puska, M.; Rantala, T. T.; Schiøtz, J.; Thygesen, K. S.; Jacobsen, K. W. Electronic Structure Calculations with GPAW: A Real-space Implementation of the Projector Augmented-wave Method. *J. Phys. Condens. Matter.* **2010**, *22*, 253202, DOI: 10.1088/0953-8984/22/25/253202.

(17) Wellendorff, J.; Lundgaard, K. T.; Møgelhøj, A.; Petzold, V.; Landis, D. D.;

Nørskov, J. K.; Bligaard, T.; Jacobsen, K. W. Density Functionals for Surface Science: Exchange-correlation Model Development with Bayesian Error Estimation. *Phys. Rev. B* **2012**, *85*, 235149, DOI: 10.1103/PhysRevB.85.235149.

(18) Garlyyev, B.; Xue, S.; Watzele, S.; Scieszka, D.; Bandarenka, A. S. Influence of the Nature of the Alkali Metal Cations on the Electrical Double-layer Capacitance of Model Pt(111) and Au(111) Electrodes. *J. Phys. Chem. Lett.* **2018**, *9*, 1927–1930, DOI: 10.1021/acs.jpclett.8b00610.

(19) Kolb, D.; J., S. Surface Reconstruction in Electrochemistry: Au(100)-(5×20), Au(111)-(1×23) and Au(110)-(1×2). *Electrochim. Acta* **1986**, *31*, 929–936, DOI: 10.1016/0013-4686(86)80005-6.

(20) Trasatti, S.; Lust, E. In *Modern Aspects of Electrochemistry*; White, R. E., Bockris, J. O., Conway, B. E., Eds.; Springer US: Boston, MA, 1999; pp 1–215, DOI: 10.1007/0-306-46917-0_1.
